# Supplementary material for: Sublinear Time and Space Algorithms for Correlation Clustering via Sparse-Dense Decompositions
Source: arXiv:2109.14528 source file (2021-09-29)
Supplement: Supplementary file 1 [file appendix-tech.tex]

% !TeX root = main.tex 
%!TEX root = main.tex

\section{Technical Preliminaries}
\label{sec:appdix-tech}
We introduce some standard technical tools we adopted in the proofs of our results in this section.
